# Supplementary material for: From a distance: Shuttleworth revisited
Source: arXiv:2311.01896 ancillary file (2024-05-15)
Supplement: Supplementary file 1 [file Supplementary_Soft_Matter.pdf]

Soft Matter

ARTICLE TYPE

Cite this: DOI: 00.0000/xxxxxxxxxx

# Supplementary Material
# From a distance: Shuttleworth revisited

Stefanie Heyden*[a] and Nicolas Bain*[b]

Received Date
Accepted Date

DOI: 00.0000/xxxxxxxxxx

## 1 Surface Projection

To project fields defined over the domain $\Omega_0$ onto the surface $S_0$, we introduce the surface projection tensor for a tangent surface with outward unit normal $\boldsymbol{N}$ as

$$\mathbb{P} = \boldsymbol{I} - \boldsymbol{N} \otimes \boldsymbol{N}, \tag{S.1}$$

where $\boldsymbol{I}$ is the second-order identity tensor[1]. A smooth vector field $\boldsymbol{v}$ (e.g. a displacement field) and a smooth second-order tensor field $\boldsymbol{T}$ (e.g. a stress field) are projected onto the surface as

$$\boldsymbol{v}_s = \mathbb{P}\boldsymbol{v} \quad \text{and} \quad \boldsymbol{T}_s = \mathbb{P}\boldsymbol{T}\mathbb{P}. \tag{S.2}$$

Furthermore, the surface gradient of a vector field follows from

$$\boldsymbol{\nabla}_s\boldsymbol{\phi} = \mathbb{P}\boldsymbol{\nabla}\boldsymbol{\phi} \quad \text{and} \quad \boldsymbol{\nabla}_s\boldsymbol{v} = (\boldsymbol{\nabla}\boldsymbol{v})\mathbb{P}. \tag{S.3}$$

As an example, the surface deformation gradient follows as

$$\boldsymbol{F}_s = \boldsymbol{I} + \mathbb{P}\nabla_s\boldsymbol{u}. \tag{S.4}$$

Note that within the manuscript, the projection tensor is dropped for simplicity as in previous studies[1].

## 2 Finite Kinematics

### 2.1 General setting

The non-linear Shuttleworth equations correspond to the expressions of the stress measures as a function of the surface energy in the current configuration $W^c$. In this setting, the second Piola-Kirchhoff stress follows as

$$\boldsymbol{S}_s = W^c \frac{\partial J_s}{\partial \boldsymbol{E}_s} + J_s \frac{\partial W^c}{\partial \boldsymbol{E}_s}. \tag{S.5}$$

[a] ETH Zürich, Institute for Building Materials, 8093 Zürich, Switzerland. E-mail: stefanie.heyden@mat.ethz.ch
[b] Universite Claude Bernard Lyon 1, CNRS, Institut Lumière Matière, UMR5306, F-69100, Villeurbanne, France. E-mail: nicolas.bain@cnrs.fr
∗ These two authors contributed equally.

Noting that $J_s = \det(\boldsymbol{F}_s) = \sqrt{\det(2\boldsymbol{E}_s + \boldsymbol{I})}$, and using the relationship

$$\frac{\partial \det \boldsymbol{M}}{\partial \boldsymbol{M}} = (\det \boldsymbol{M})\boldsymbol{M}^{-T} \tag{S.6}$$

for any invertible tensor $\boldsymbol{M}$, we obtain the non-linear Shuttleworth equation for the second Piola-Kirchhoff stress tensor

$$\boldsymbol{S}_s = W^c J_s \left(\boldsymbol{F}_s^{\mathrm{T}}\boldsymbol{F}_s\right)^{-1} + J_s \frac{\partial W^c}{\partial \boldsymbol{E}_s}. \tag{S.7}$$

Equivalently, the first Piola-Kirchhoff stress tensor reads

$$\boldsymbol{P}_s = W^c J_s \boldsymbol{F}_s \left(\boldsymbol{F}_s^{\mathrm{T}}\boldsymbol{F}_s\right)^{-1} + J_s \boldsymbol{F}_s \frac{\partial W^c}{\partial \boldsymbol{E}_s}, \tag{S.8}$$

and the Cauchy stress is given as

$$\boldsymbol{\sigma}_s = W^c \mathbf{I} + \boldsymbol{F}_s \frac{\partial W^c}{\partial \boldsymbol{E}_s} \boldsymbol{F}_s^{\mathrm{T}}. \tag{S.9}$$

### 2.2 Surface stress-strain relations

We can tailor stress measures to a specific constitutive material model by choosing, e.g., the St. Venant-Kirchhoff model

$$W^R(\boldsymbol{E}_s) = \gamma J_s + \mu_s \operatorname{tr}(\boldsymbol{E}_s\boldsymbol{E}_s) + \frac{1}{2}\lambda_s (\operatorname{tr}(\boldsymbol{E}_s))^2. \tag{S.10}$$

In addition to relation (S.6), we note that the derivative of a tensor $\boldsymbol{M}$ with respect to that tensor is simply $\frac{\partial \operatorname{tr}(\boldsymbol{M})}{\partial \boldsymbol{M}} = \boldsymbol{I}$. Using the chain rule, the different stress measures under consideration then follow as

$$\begin{aligned} \boldsymbol{S}_s = \frac{\partial W^R}{\partial \boldsymbol{E}_s} &= \boldsymbol{F}^{-1} \frac{\partial W^R}{\partial \boldsymbol{F}_s} \\ &= \gamma J_s (\boldsymbol{F}_s^T \boldsymbol{F}_s)^{-1} + 2\mu_s \boldsymbol{E}_s + \lambda_s \operatorname{tr}(\boldsymbol{E}_s)\boldsymbol{I}, \end{aligned} \tag{S.11}$$

and the relations

$$\boldsymbol{P}_s = \boldsymbol{F}_s\boldsymbol{S}_s \text{ and } \boldsymbol{\sigma}_s = J_s^{-1}\boldsymbol{P}_s\boldsymbol{F}_s^T \tag{S.12}$$

lead to the main text equations (7) and (8).

## 3 Linearization

For linearized surface relaxation, we express all quantities at play, $J$, $\boldsymbol{F}$ and $\boldsymbol{E}$ at first order in displacement gradient $\boldsymbol{\nabla u}$ or in strains $\boldsymbol{\varepsilon}$. The deformation gradient is readily defined at first order, $\boldsymbol{F} = \boldsymbol{I} + \boldsymbol{\nabla u}$, the Green-Lagrange strain tensor at first order simplifies to the linear strains $\boldsymbol{E} = \boldsymbol{\varepsilon} + \mathscr{O}(\boldsymbol{\varepsilon}^2)$, and the local area change simplifies to $J = [1 + \mathrm{tr}(\boldsymbol{\varepsilon})] + \mathscr{O}(\boldsymbol{\varepsilon}^2)$.

For finite surface relaxation, we expand all terms to linear order in $\boldsymbol{\nabla u}^0$, whereas terms involving $\boldsymbol{F}^*$ stay finite. The deformation gradient then simplifies to $\boldsymbol{F} = (\boldsymbol{I} + \boldsymbol{\nabla u}^0)\boldsymbol{F}^* + \mathscr{O}([\boldsymbol{\nabla u}^0]^2)$, the Green-Lagrange tensor to $\boldsymbol{E} = \boldsymbol{E}^* + \boldsymbol{F}^*\boldsymbol{\varepsilon}^0(\boldsymbol{F}^*)^T + \mathscr{O}([\boldsymbol{\nabla u}^0]^2)$, and the local area change to $J = \left[1 + \mathrm{tr}(\boldsymbol{\varepsilon}^0)\right] J^* + \mathscr{O}(\boldsymbol{\varepsilon}^2)$.

## 4 Finite surface relaxation in the absence of surface shear

In the absence of surface shear, the surface deformation gradient is diagonal

$$\mathbf{F}_{\mathrm{s}} = \begin{pmatrix} F_{\mathrm{s}\parallel} & 0 \\ 0 & F_{\mathrm{s}\perp} \end{pmatrix}, \tag{S.13}$$

with $F_{\mathrm{si}} = 1 + \varepsilon_{\mathrm{si}}$, where $i = \parallel$ or $i = \perp$ denote the two principal directions. Assuming the principal directions of the surface relaxation and of the imposed deformation coincide, we obtain the generic expression for the Cauchy principal stresses

$$\begin{aligned} \bar{\sigma}_{\mathrm{si}} =& \gamma + \bar{\sigma}^*_{\mathrm{si}} + 2\mu_{\mathrm{s}} \left( (F^*_{\mathrm{si}})^4 + 2(F^*_{\mathrm{si}})^2 E^*_{\mathrm{si}} \right) \varepsilon^0_{\mathrm{si}} \\ &+ \lambda_{\mathrm{s}} \left( (F^*_{\mathrm{si}})^4 + 2(F^*_{\mathrm{si}})^2 (E^*_{\mathrm{si}} + E^*_{\mathrm{sj}}) \right) \varepsilon^0_{\mathrm{si}} \\ &+ \lambda_{\mathrm{s}} (F^*_{\mathrm{si}} F^*_{\mathrm{sj}})^2 \varepsilon^0_{\mathrm{sj}}, \end{aligned} \tag{S.14}$$

with $(i,j) = (\parallel,\perp)$ or $(i,j) = (\perp,\parallel)$ the principal directions, $\bar{\sigma}^*_{\mathrm{si}} = (2\mu_{\mathrm{s}} + \lambda_{\mathrm{s}})(F^*_{\mathrm{si}})^2 E^*_{\mathrm{si}} + \lambda_s (F^*_{\mathrm{si}})^2 E^*_{\mathrm{sj}}$ the surface relaxation stress contribution and $E_{\mathrm{si}} = \varepsilon_{\mathrm{si}}(2 + \varepsilon_{\mathrm{si}})/2$ the diagonal components of the Green-Lagrange strain tensor.

## 5 Relaxing cylinder

The total energy of the relaxing cylinder,

$$W_{\mathrm{tot}} = \min_{\lambda^*} \left( S_0\,\gamma + V_0\,W^{\mathrm{R}}(\lambda^*) \right), \tag{S.15}$$

comprises a surface contribution $S_0\,\gamma$ and a bulk contribution $V_0\,W^{\mathrm{R}}(\lambda^*)$, where $S_0$ and $V_0$ are the surface and volume of the relaxed cylinder, respectively. Here, $W^{\mathrm{R}}(\lambda^*) = \mu(2\lambda^{*2} + \lambda^{*-4} - 3)/2$ derives from the strain energy density of a Neo-Hookean incompressible material. The solutions to Eq. (S.15) are

$$\lambda^{*3}_{\pm} = \frac{\gamma/R \pm \sqrt{(\gamma/R)^2 + 4\mu^2}}{4\mu}, \tag{S.16}$$

from which we discard $\lambda^*_-$ for physical reasons ($\lambda^* > 0$ when $L_{ec}/R \ll 1$), which leads to Eq. (19).

## Notes and references


1 S. Krichen, L. Liu and P. Sharma, *JMPS*, 2019, **127**, 332–357.
